# Supplementary material for: Semantic Relational Object Tracking
Source: arXiv:1902.09937 source file (2019-02-26)
Supplement: Supplementary file 1 [file appendix_dc.tex]

\section{Dynamic Distributional Clauses}\label{app:ddc}

\begin{example}\label{dc_example}
In order to exemplify the expressive power of DC we give an example program with continuous and discrete random variables:
\begin{addmargin}{1em}
\vspace*{-\baselineskip}
\begin{flalign}
& \mathtt{n} \sim \mathtt{poisson}(6).&\\
&\mathtt{pos}(\mathtt{P})\sim \mathtt{uniform}(0,\mathtt{N})\leftarrow & \nonumber \\
& \qquad \mathtt{N}\sim = \mathtt{n}, \mathtt{between}(1,\mathtt{N}, \mathtt{P}). &\\
&\mathtt{left}(\mathtt{A},\mathtt{B}) \sim \mathtt{finite}([0.99:\mathtt{t},0.01:\mathtt{f}])\leftarrow & \nonumber \\
&\qquad \mathtt{P1}\sim = \mathtt{pos}(\mathtt{A}), \mathtt{P2}\sim = \mathtt{pos}(\mathtt{B}), \mathtt{P1}<\mathtt{P2}.&
\end{flalign}
\end{addmargin}
In this program, we describe a scenario where we have a number of $\mathtt{n}$ objects, where this number is distributed according to a Poisson distribution with mean $6$. We then define a position for each object by using the built-in $\mathtt{between}$ predicate which evaluates to $\mathtt{true}$ if $1\leq\mathtt{P}\leq\mathtt{N}$. $\mathtt{N}$ unifies with the value of $\mathtt{n}$, which is an integer sampled from the Poisson distribution. The last line gives us the probability of an object $\mathtt{A}$ being to the left of a object $\mathtt{B}$. $\mathtt{left(1,2)}$ for example, can take the values $\mathtt{t}$ ($\mathtt{true}$) or $\mathtt{f}$ ($\mathtt{false}$) with a certain probability.
\end{example}

Example~\ref{dc_example} demonstrates how the real world can easily be modeled through the means of probabilistic relational clauses. However, agents and objects do not only occupy a position in the $3{\text -}D$ physical world but do also travel in time, therefore we need an explicit dependency on time that facilitates the description of dynamics. It is here where Dynamic DC comes into play. Labeling random variables with time indices gives us the temporal component. Example~\ref{ddc_example} demonstrates how a transition from one time step to the next can be defined. 

\begin{example}\label{ddc_example}
Labeling random variables with a time index allows to define the dynamics present in the world. We can for instance define how the position of an object evolves over time:
\begin{addmargin}{1em}
\vspace*{-\baselineskip}
\begin{flalign}
&\mathtt{n} \sim \mathtt{poisson}(6).&\\
&\mathtt{pos}(\mathtt{P})_0\sim \mathtt{uniform}(0,\mathtt{N})\leftarrow& \nonumber \\
& \qquad \mathtt{N}\sim = \mathtt{n}, \mathtt{between}(1,\mathtt{N}, \mathtt{P}).&\\
&\mathtt{pos}(\mathtt{P})_{t+1} \sim \mathtt{gaussian}(\mathtt{X}+3, \Sigma)\leftarrow& \nonumber \\
& \qquad \mathtt{X}\sim = \mathtt{pos}(\mathtt{P})_t.&
\end{flalign}
\end{addmargin}
This program defines in the first line the number of objects present in the world, then initializes the position for each of the objects, and finally describes how the position evolves over time: at each time step the object moves three units of length, giving it a velocity of $3\text{ }[length]/[time]$.
\end{example}
